# Supplementary material for: s-wave superconductivity in kagome metal CsV$_{3}$Sb$_{5}$ revealed by $^{121/123}$Sb NQR and $^{51}$V NMR measurements
Source: arXiv:2104.06698 source file (2021-07-02)
Supplement: Supplementary file 1 [file Supplement.pdf]

Supplemental Material for

# *s*-wave superconductivity in kagome metal $CsV_3Sb_5$ revealed by $^{121/123}$Sb NQR and $^{51}$V NMR measurements

Chao Mu,[1,2] Qiangwei Yin,[3] Zhijun Tu,[3] Chunsheng Gong,[3] Hechang Lei,[3] Zheng Li,[1,2,] and Jianlin Luo[1,2,4]
[1]Beijing National Laboratory for Condensed Matter Physics and Institute of Physics, Chinese Academy of Sciences, Beijing 100190, China
[2]School of Physical Sciences, University of Chinese Academy of Sciences, Beijing 100190, China
[3]Department of Physics and Beijing Key Laboratory of Opto-electronic Functional Materials & Micro-nano Devices, Renmin University of China, Beijing 100872, China
[4]Songshan Lake Materials Laboratory, Dongguan 523808

## 1. Knight shift and spin-lattice relaxation rate of $^{51}$V with $H \perp c$

Figure S1 shows $^{51}K$ jumps up below $T_{CDW}$ with $H \perp c$, however $^{51}(1/T_1T)$ for both directions does not jump up. It indicates that the splitting and jumping of $^{51}K$ at $T_{CDW}$ are not by the change of hyperfine coupling constants, but by the orbital part of Knight shift.

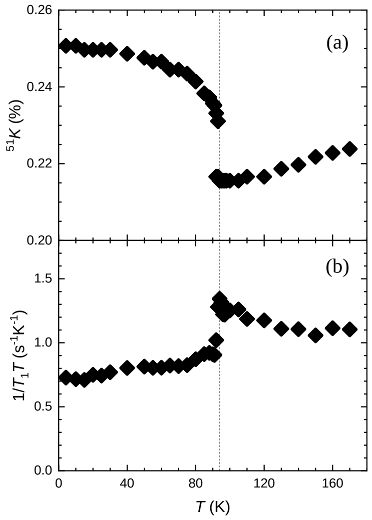


Fig. S1. (a) Temperature dependence of the Knight shift of $^{51}$V. (b) Temperature dependence of the $^{51}(1/T_1T)$. The vertical dashed line indicates the position of $T_{CDW}$.

## 2. Sb spectra

There are two different crystallographic sites of Sb in $CsV_3Sb_5$. Sb1 atoms locate in the kagome plane with V atoms and Sb2 atoms encapsulate the kagome layer with a graphitelike network. The atomic ratio is Sb1 : Sb2 = 1 : 4, which determines the spectra intensity ratio. Therefore, we can distinguish two Sb spectra by their peak intensity. Fig. S2 shows the spectrum from 67 MHz to 161 MHz at 4.2 K.

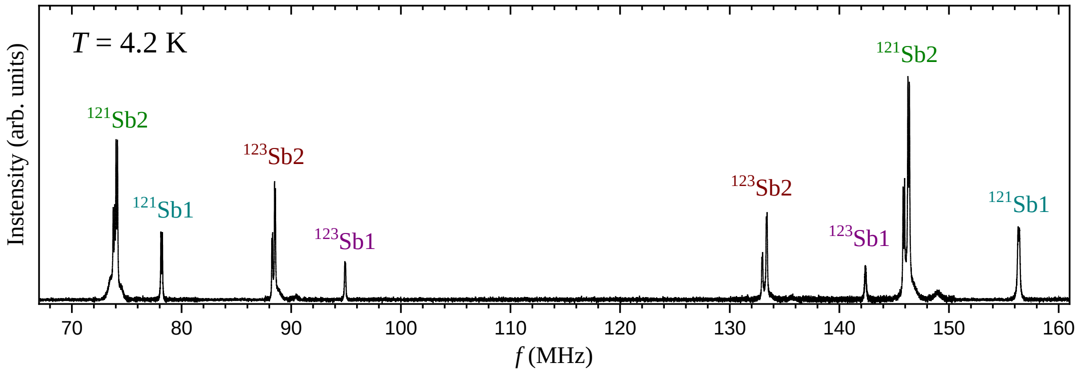


Fig. S2. $^{121/123}$Sb-NQR spectra with a perturbing field of 64 Oe along $c$-axis at 4.2 K.

The peaks of Sb1 atoms are shown in Fig. S3. Below $T_{CDW}$ = 94 K, peaks shift to higher frequency which indicates EFG strength increases. The pairing of peaks at 4.2 K is due to a perturbing field of 64 Oe along *c*-axis. They merge together when peaks are broad at 130 K.

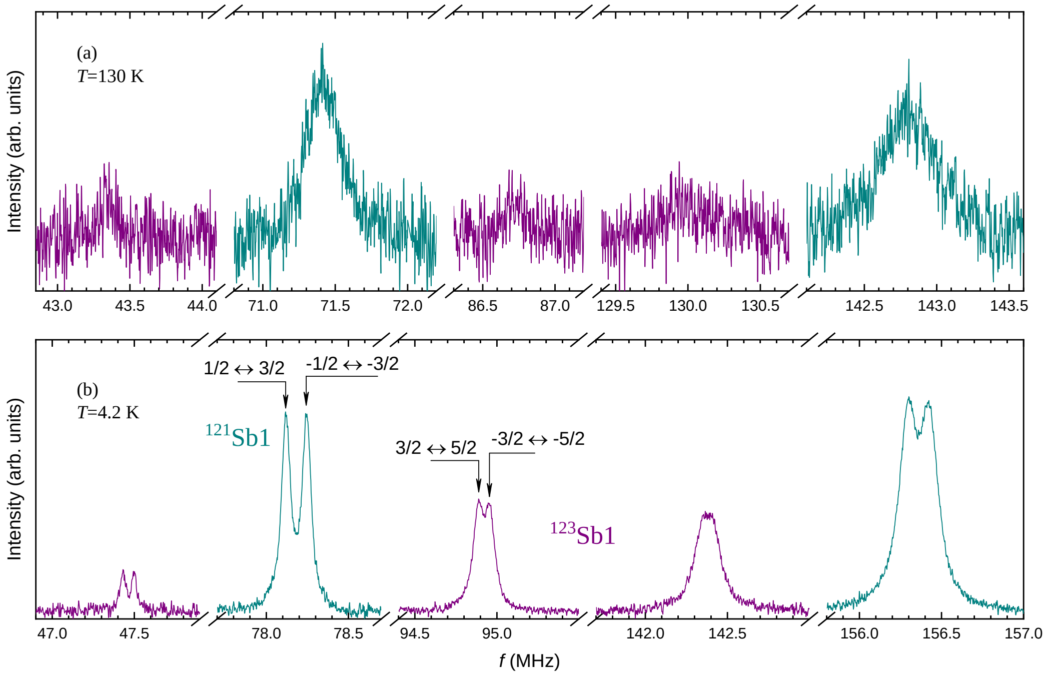


Fig. S3. (Color online) $^{121/123}$Sb1-NQR spectra with a perturbing field of 64 Oe along *c*-axis at (a) 130 K and (b) 4.2 K respectively.

The change of EFG is different between Sb1 site and Sb2 sites below $T_{CDW}$. The EFG strength is enhanced without asymmetry at Sb1 site in the kagome plane. On the other hand, the main change is not the EFG strength, but the EFG direction at Sb2 sites out of kagome plane. Moreover, in the CDW state, Sb2 has two unequal sites with ratio of 1:2 from the electric field gradient point of view, while Sb1 has only one site. It imposes constraints on the possible configurations of the CDW state.

We emphasize that two Sb2 sites with ratio of 1:2 are intrinsic. There is only one set of peaks of Sb2 above $T_{CDW}$ and no other peak from impurity. Below $T_{CDW}$, the peaks of Sb2 split into two sets, which is same as that of $^{51}$V. The peaks of Sb1 do not split below $T_{CDW}$, as shown in Fig. S3 (b), so the splitting of Sb2 is not from defects. Otherwise, both Sb1 and Sb2 should split at the same time. The ratio of 1:2 is also an indirect proof that it is intrinsic. Defects induced peaks should have an arbitrary ratio and the ratio should change with temperature. Moreover, the full width at half maximum (FWHM) of two splitting peaks are same, which proves they are all intrinsic.
